# Supplementary material for: Electron-hole symmetry in quasiparticle spectral weight of cuprates observed via infrared and photoemission spectroscopy
Source: arXiv:2203.07575 source file (2022-03-15)
Supplement: Supplementary file 1 [file Electron-hole_symmetry_Supplementary_Information_JH.pdf]

Supplementary Information

# Electron-hole symmetry in quasiparticle spectral weight of cuprates observed via infrared and photoemission spectroscopy

Myounghoon Lee[1,+], Dongjoon Song[2,3,+], Yu-Seong Seo[1], Seulki Roh[1], Seokbae Lee[1], Hiroshi Eisaki[3], and Jungseek Hwang[1*]

[1]*Department of Physics, Sungkyunkwan University, Suwon, Gyeonggi-do 16419, Republic of Korea*

[2]*Center for Correlated Electron Systems, Institute for Basic Science (IBS), Seoul 08826, Republic of Korea*

[3]*National Institute of Advanced Industrial Science and Technology, Tsukuba 305-8568, Japan*

* Electronic address: jungseek@skku.edu

[+] These authors contributed equally to this work.

## Superconducting transition of PLCCO samples observed by magnetic susceptibility measurements

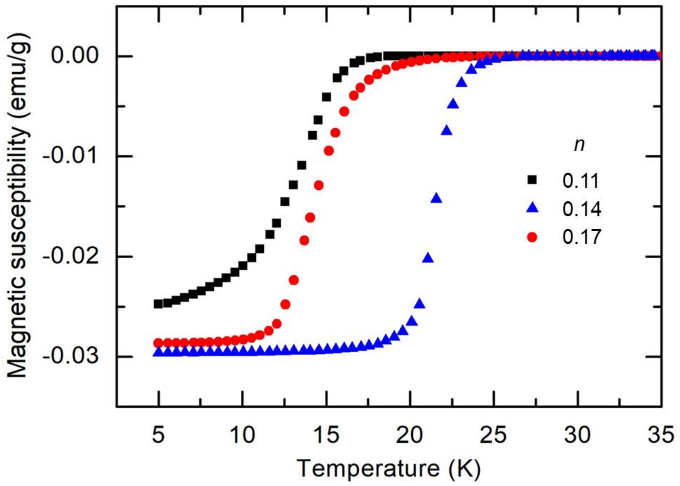


**Figure S1.** Magnetic susceptibility of superconducting PLCCO samples measured by a zero-field cool method. A 10 Oe magnetic field was applied along the *c*-axis of the samples. The 10 % of the shielding volume fractions are determined as the superconducting transition temperatures ($T_c$), which correspond to 15 K ($n$ = 0.11), 24 K ($n$ = 0.14), and 18 K ($n$ = 0.17), respectively.

## Reflectance spectra of PLCCO samples at various temperatures

The measured reflectance spectra of the four PLCCO single-crystal samples at various temperatures are shown in Fig. S2 (a)-(d). All four samples show metallic behavior. The reflectance in the far-infrared (FIR) region below 800 $cm^{-1}$ increases with decreasing temperature. In the mid-infrared (MIR) region, the well-known antiferromagnetic pseudogap feature appears as a slightly suppressed reflectance between 1000 and 3000 $cm^{-1}$ [S1] compared to the reflectance at 300 K, at which the pseudogap is closed. The plasma edge, which appears as a dip near 8000 $cm^{-1}$, occurs at a lower frequency than those (~10,000 $cm^{-1}$) observed in the PCCO and NCCO systems.

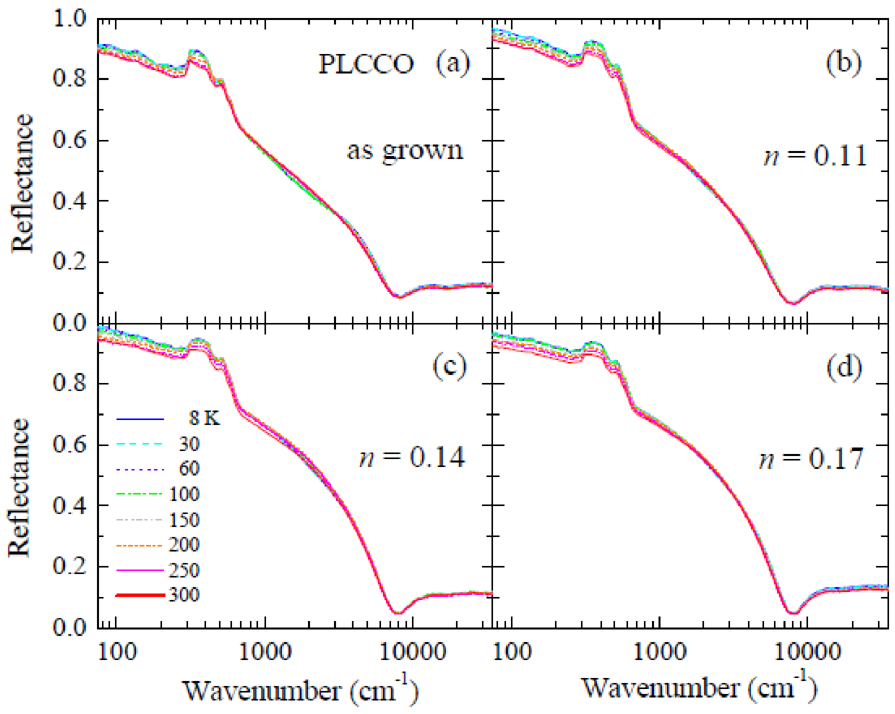


**Figure S2.** Measured reflectance spectra of four PLCCO samples: (a) as-grown, (b) $n$ = 0.11, (c) $n$ = 0.14, and (d) $n$ = 0.17 at various selected temperatures across a wide spectral range from 75 to 35,000 $cm^{-1}$.

## Miscut from the *ab* plane checked using optical measurements and Laue patterns

We checked how accurately the samples were cut along the *ab* plane in a simple experiment using a polarizer and confirmed that miscut effects in the measured reflectance spectra were negligibly small (see Fig. S3). Fig. S3 shows the reflectance spectra of the cut and polished surfaces of all four samples at various angles of linear polarization with respect to a reference angle, which gives the maximum reflectance. We note that we measure both the reflectance

spectra of the sample and a reference mirror at each polarizer angle to avoid the slightly polarized light source. The reflectance is maximum at 0° and is minimum at 90°. The difference between the maximum and minimum is around 2.5% and no additional significant phonon features appear in the measured reflectance spectra, indicating the cut and polished surface is close to the *ab* plane. If the surface is significantly miscut from the *ab* plane the strong *c*-axis phonons are expected to appear in the measured reflectance at a certain angle. Additionally, we performed the Laue measurements and found that the cut and polished surface is very close to the *ab* plane. We show the measured Laue patterns of our four samples in the insets of Fig. S2. From the Laue patterns, we obtained the miscut angles of around 4°, 2°, 5° and 2° for the as-grown, $n$ = 0.11, 0.14 and 0.17 samples, respectively.

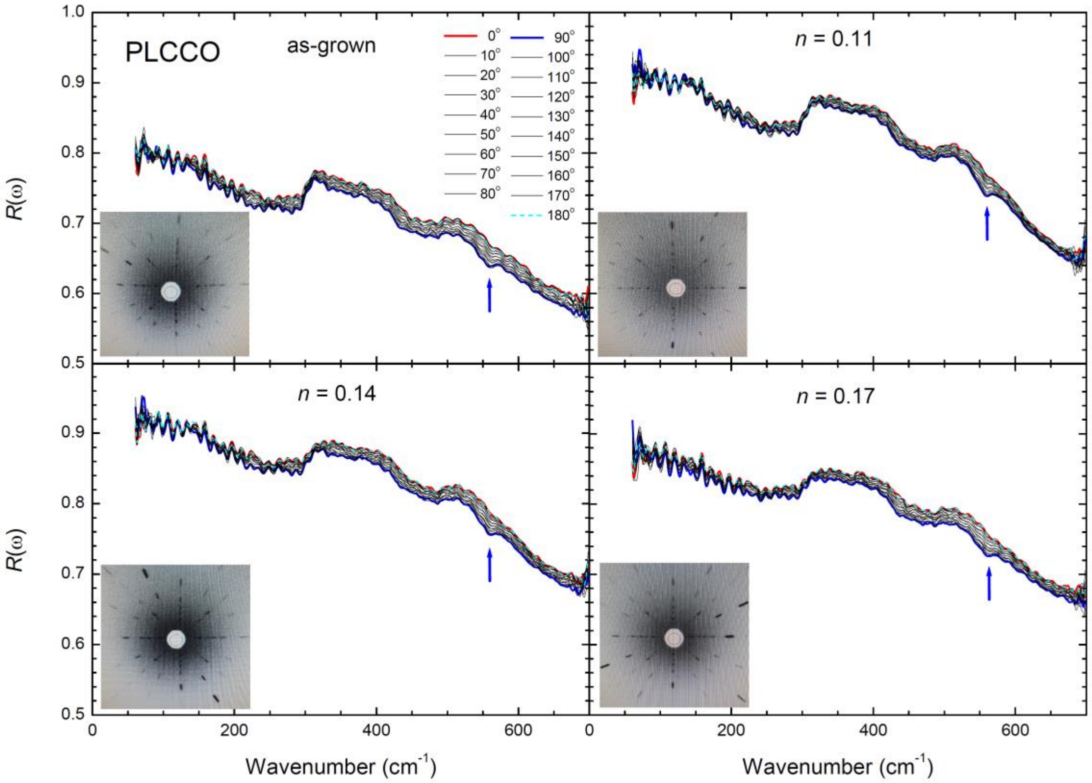


**Figure S3.** Measured reflectance spectra of the cut and polished surfaces of our four samples at 300 K with various polarization angles with respect to the *ab* plane. In the inset, the Laue patterns of the corresponding surfaces are shown.

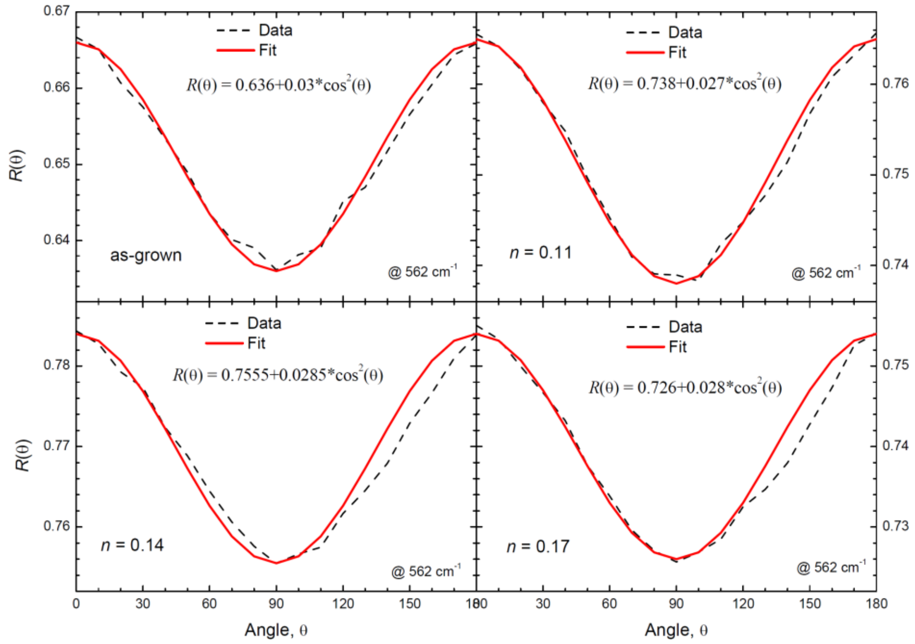


**Figure S4.** The reflectance data at 562 $cm^{-1}$ (marked with blue arrows in Fig. S2) as functions of the polarization angles and fits with a periodic function, $(I_{max} - I_{min}) \cos^2\theta + I_{min}$, where $I_{max}$ is the maximum value at $\theta = 0°$ and $I_{min}$ is the minimum value at $\theta = 90°$ at 562 $cm^{-1}$.

Fig. S4 shows the reflectance data and fits of the four samples at 562 $cm^{-1}$ as functions of the polarization angle. We can observe a periodic change in the reflectance data as a function of $\theta$ with a period of 180°. It is worth noting that since the incident angle is about 11° the anisotropic contribution from the deviation from the normal incidence is added to the measured angle-dependent reflectance data. Therefore, the actual miscut can be smaller than the angle estimated from the angle-dependent reflectance data.

## References


[S1] Y. Onose, Y. Taguchi, K. Ishizaka, and Y. Tokura, Charge dynamics in underdoped $Nd_{2-x}Ce_xCuO_4$: Pseudogap and related phenomena *Phys. Rev. B* **69**, 024504 (2004).
